# Supplementary material for: Hydrogenated-Graphene encapsulated Graphene: A versatile material for device applications
Source: arXiv:1905.03965 source file (2019-10-04)
Supplement: Supplementary file 1 [file Supporting_information_compressed.pdf]

# Supplementary Material: Hydrogenated-Graphene encapsulated Graphene: A versatile material for device applications

Mohammed Ghadiyali, Sajeev Chacko

*Department of Physics, University of Mumbai, Kalina Campus, Santacruz (E), Mumbai - 400 098, India.*

## 1. Hydrogenated graphene / graphene trilayer systems

The atomic positions for the systems under the study has been given in the crystal coordinates as described in Quantum ESPRESSO

### 1.1. The System A0

```
C  0.98624100  0.97199200  0.38396300
C  0.00332637  0.00419736  0.49992000
C  0.31903000  0.63800000  0.39724900
C  0.66956900  0.33701300  0.49992200
C  0.01304290  0.02697150  0.61537400
C  0.34589200  0.69281000  0.60207200
H  0.98613800  0.97192100  0.35225300
H  0.31919400  0.63820500  0.42888100
H  0.01286890  0.02672230  0.64708100
H  0.34596600  0.69286900  0.57044300
```

### 1.2. The System A60

```
C -0.003064523  0.003035392  0.379415435
C  0.012181497 -0.012061747  0.499895581
C  0.330571061  0.669401903  0.392717145
C  0.345034514  0.655091668  0.499893838
C -0.003195736  0.003161588  0.619905911
C  0.330428045  0.669540148  0.606641038
H -0.003027443  0.002998051  0.347709033
H  0.330500519  0.669471519  0.424359469
H -0.003141459  0.003106937  0.651609202
H  0.330378524  0.669589539  0.574995348
```

### 1.3. The System B0

```
C  0.059411285  0.025699321  0.385280275
C -0.029821211 -0.013041647  0.495116982
C  0.391842793  0.691489515  0.385276865
```

*Email addresses:* ghadiyali.mohd@physics.mu.ac.in (Mohammed Ghadiyali), sajeev.chacko@physics.mu.ac.in; sajeev.chacko@gmail.com (Sajeev Chacko)

```
C  0.636190725  0.319586925  0.508489109
C  0.001503461  0.001800019  0.611133869
C  0.334170234  0.667818876  0.611131737
H -0.029913066 -0.013126889  0.463443110
H  0.636453774  0.319797480  0.540127724
```

*1.4. The System B60*

```
C  0.081586000 -0.334210275  0.389005919
C -0.233367781  0.008314663  0.493274003
C  0.415630550  0.332813157  0.389007842
C  0.098701781  0.674348417  0.506748666
C  0.385983940  0.317994488  0.610970828
C  0.720037936  0.985022800  0.610972845
H -0.233870753  0.008068087  0.461621253
H  0.098630328  0.674316663  0.538398643
```

## 2. Band structure of Trilayer graphene encapsulated with HG

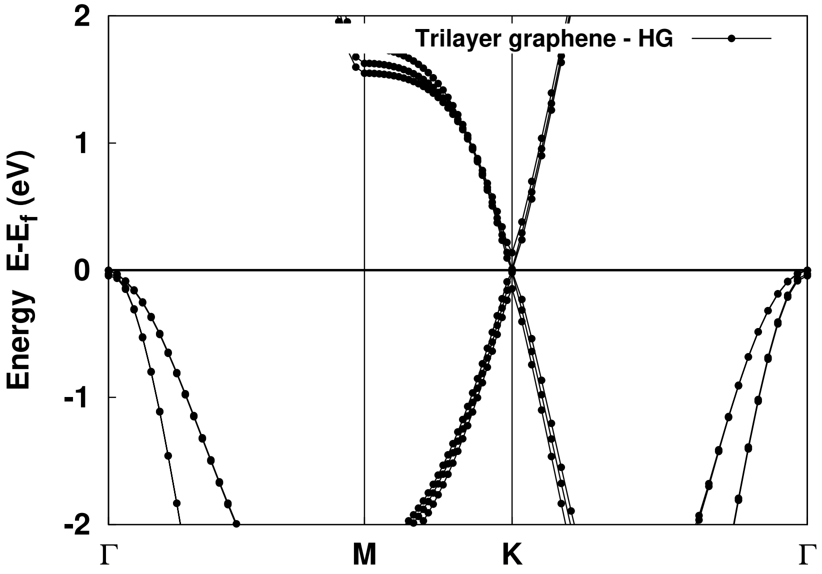


SI: 1: The image above is the band structure of trilayer graphene encapsulated by HG. It can be noted that all the necessary features of the free standing trilayer graphene has been preserved. As the physics manifestation of Z2 invariant trilayer graphene can demonstrate QSHE, hence a basic study is done where the band structure of the systems is computed.

## 3. *k*-resolved Projected Density of States

### *3.1. k-PDOS of system A0*

With the reference of the figure 2 below, one can observe that the Dirac point at the K-point has the most contribution form the carbon atoms of the graphene (figure 2(e,f)), while the states near the Γ-point originates due to the carbon and hydrogen of the HG

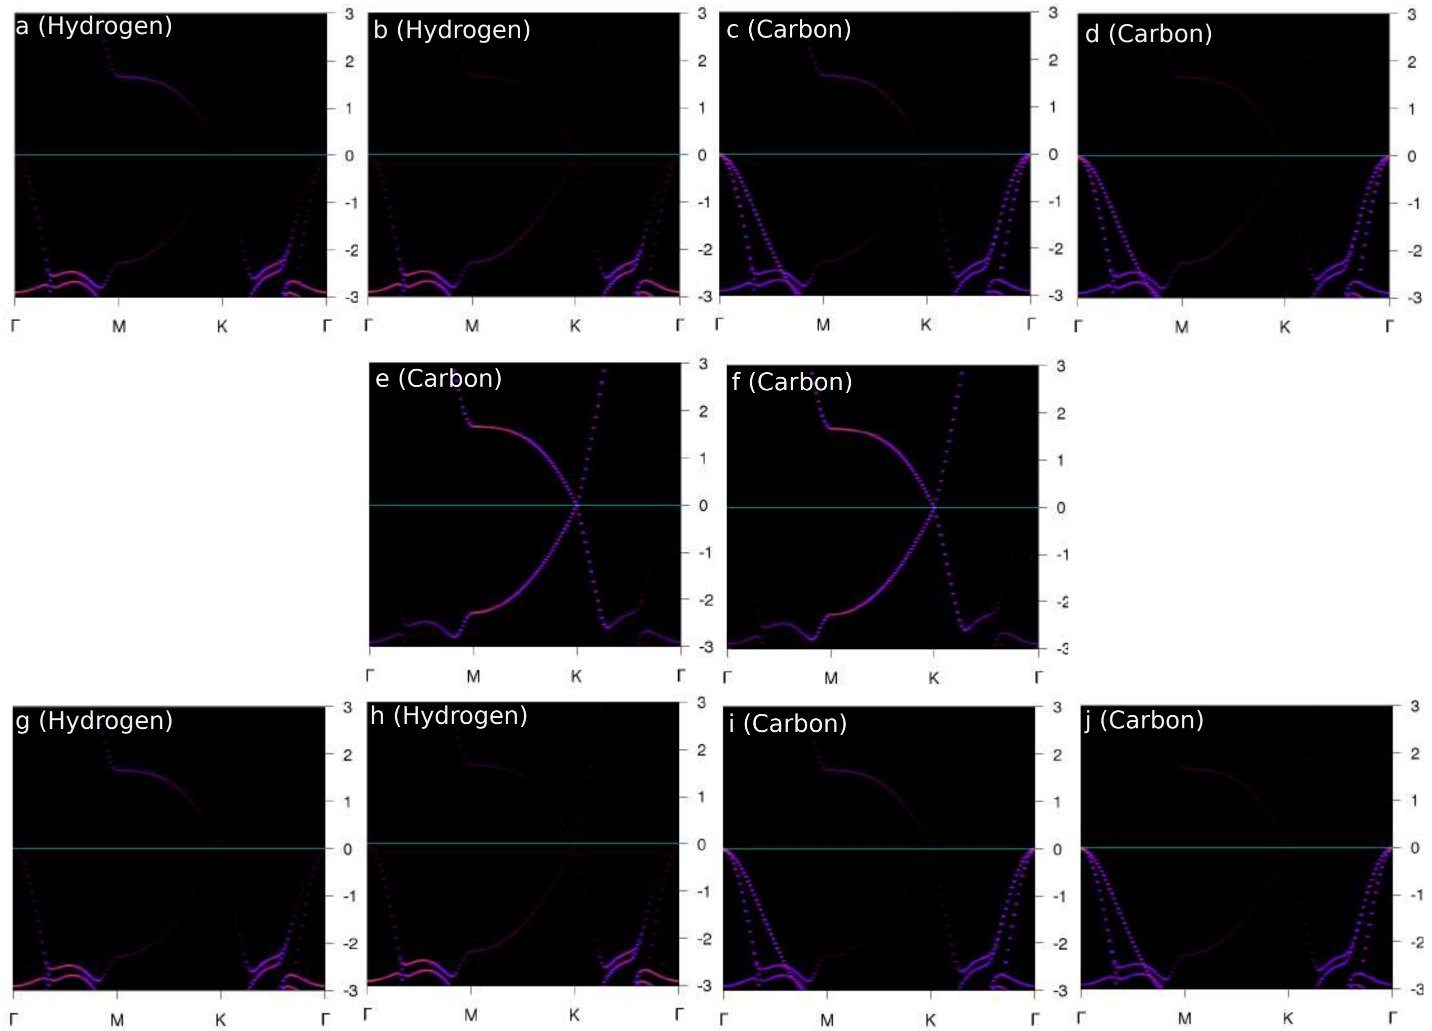


SI: 2: (colour online) The top four images (a,b,c,d) are the band structure of top HG, the middle two (e,f) are the band structure of pristine graphene and bottom four (g,h,i,j) are the band structure of the bottom HG.

*3.2. k-PDOS of system A60*

With the reference of the figure 3 below, one can observe that the Dirac point at the K-point has the most contribution form the carbon atoms of the graphene (figure 3(e,f)), while the states near the Γ-point originates due to the carbon and hydrogen of the HG

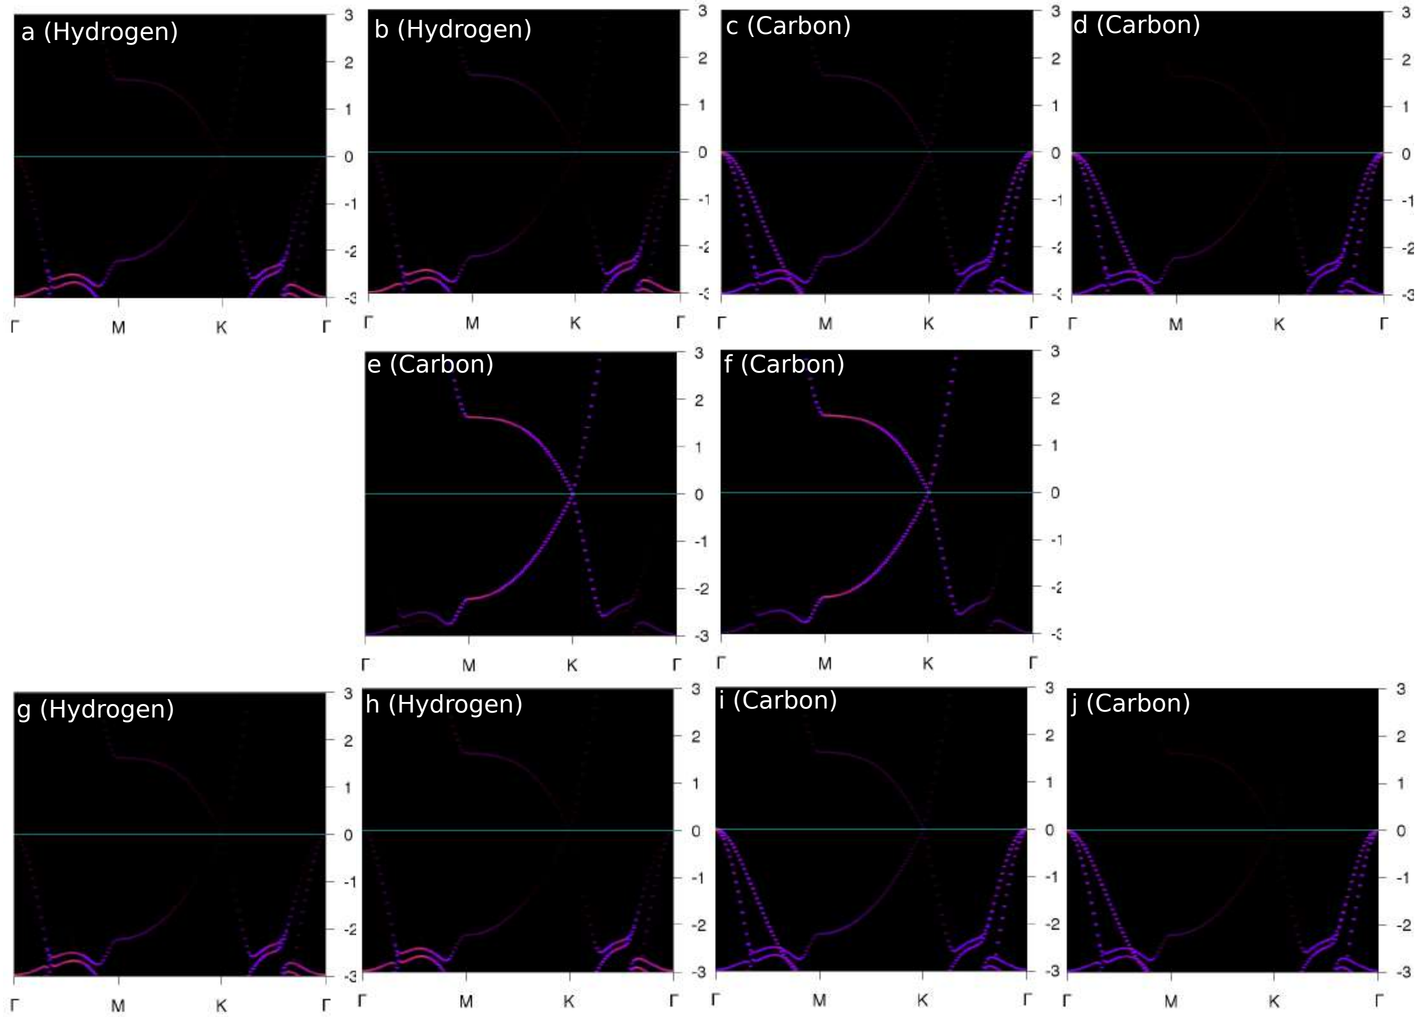


SI: 3: (colour online) The top four images (a,b,c,d) are the band structure of top HG, the middle two (e,f) are the band structure of pristine graphene and bottom four (g,h,i,j) are the band structure of the bottom HG.

### *3.3. k-PDOS of system B0*

The top two and bottom two images in figure 4 (a, b, g and h) are of the pristine graphene in the system B0. It can be noticed that the bands near the $K$-point have the major contribution form them. The middle images of figure 4 (c, d, e and f) are of the HG and the bands at the Γ-point have the major contribution from them.

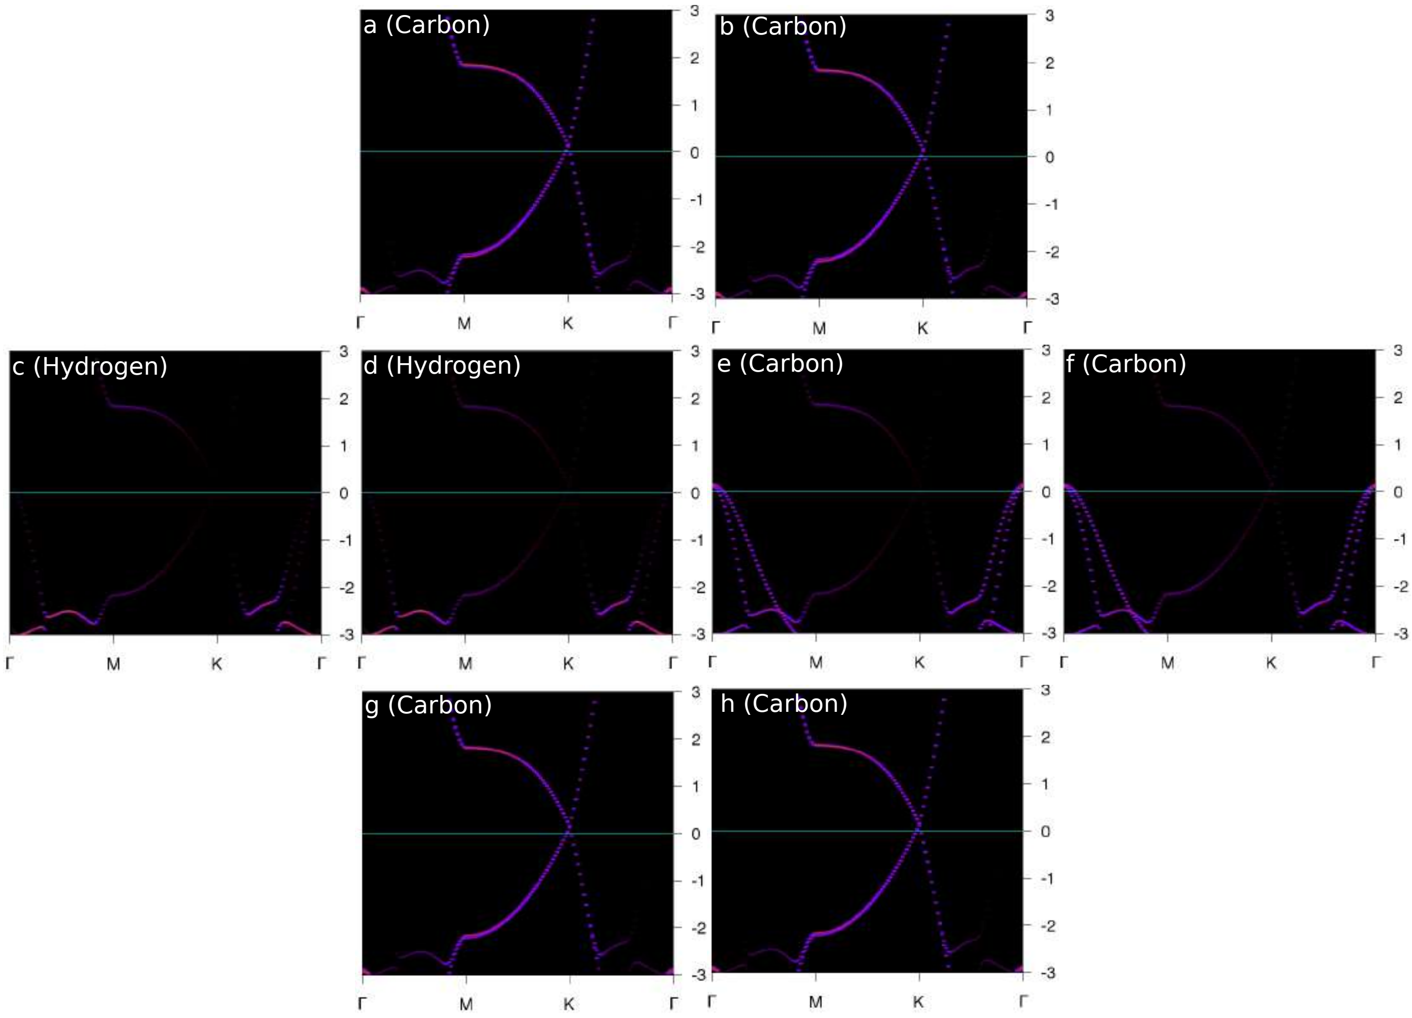


SI: 4: (colour online) The top four images (a, b, g and h) and the bottom four images (c, d, e and f) are the band structure of top and bottom pristine graphene, respectively, and the middle two images (e,f) are the band structure of central HG.

*3.4. k-PDOS of system B60*

The top two and bottom two images in figure 5 (a, b, g and h) are of the graphene in the system B0, it can be noticed that the bands near the K-point have the major contribution form them. The middle images of figure 5 (c, d, e and f) are of the HG and the bands at the Γ-point have the major contribution from them.

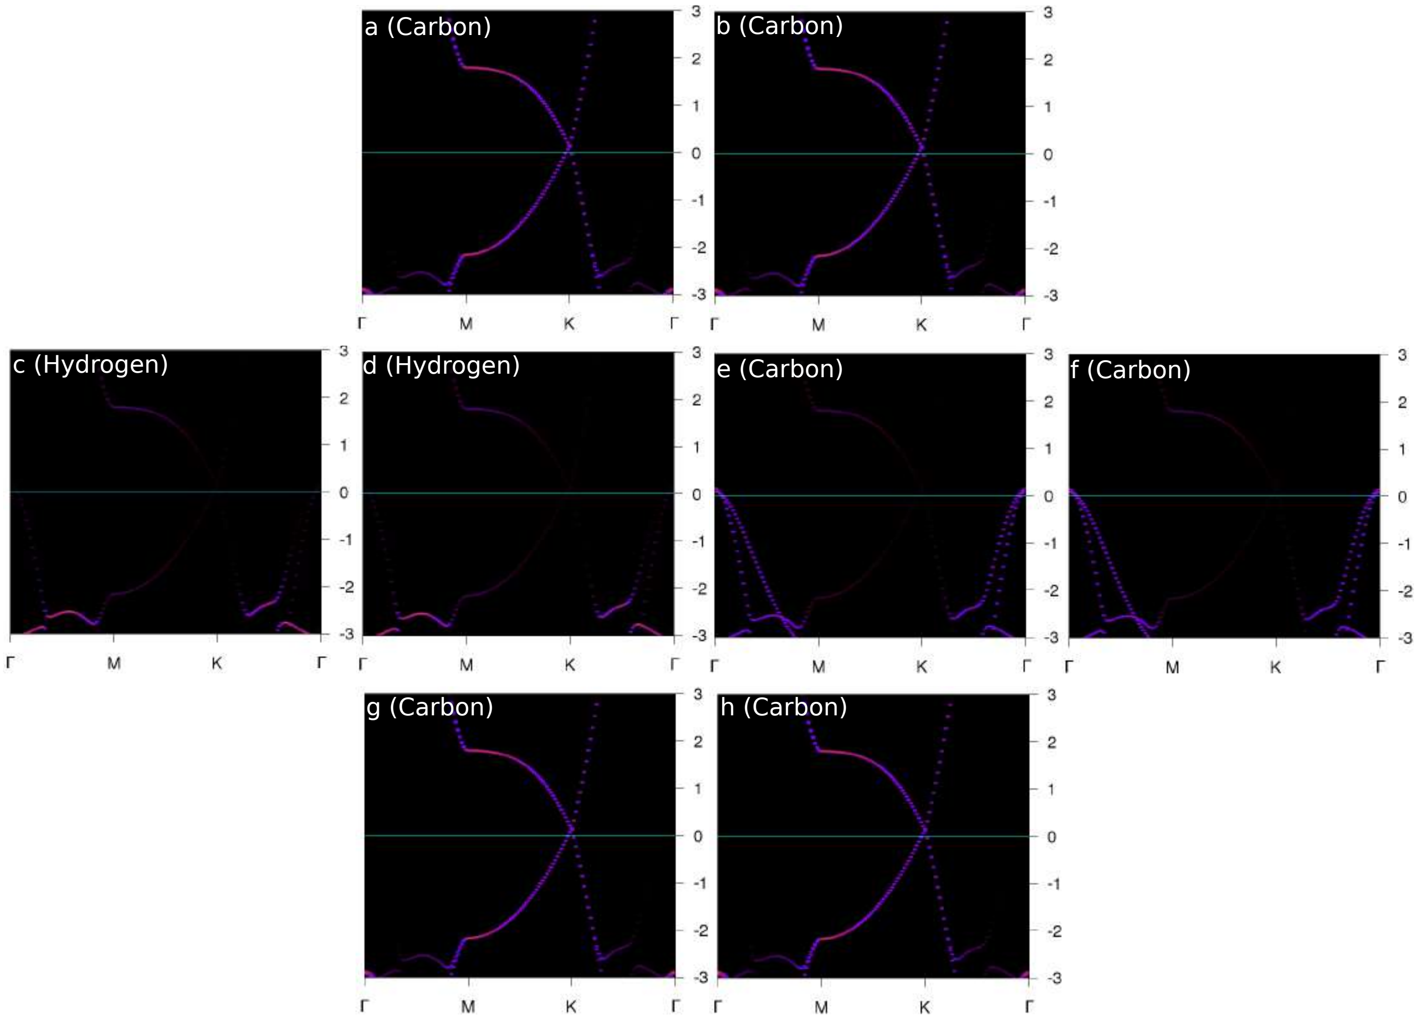


SI: 5: (colour online) The top two and bottom two (a, b, g and h) are of Graphene and the middle four (c, d, e and f) are of the HG

## 4. Charge Density

Here we have given the charge density of the system A0. As we have mentioned in the main paper, that the electronic states hydrogen atoms of hydrogenated graphene does not interfere with the electronic states of graphene. This is based on two facts one the distance between the hydrogen atoms and graphene is high so that it does not interfere. This can be observed, as the charge density between the all three layers is absent.

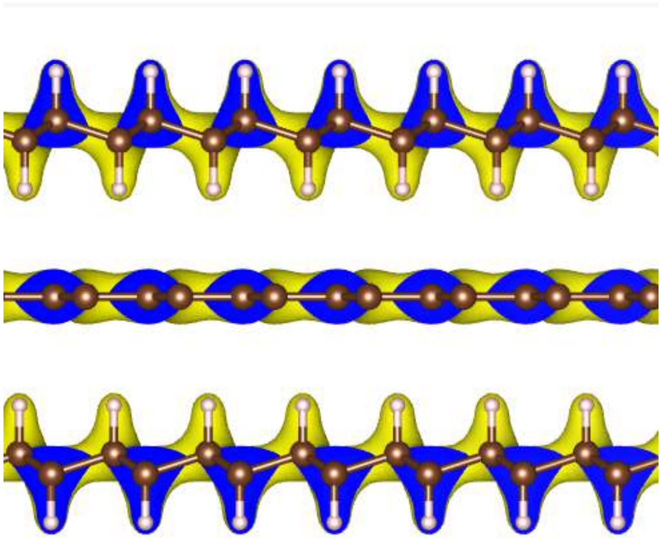

SI: 6: (colour online) System A0 band structure under positive electric field.

## 5. Selected *k*-resolved PDOS of nanoribbon

Here are the *k*-resolved PDOS of the nanoribbons, as the number of the atoms in these systems are very high, here only representative PDOS are presented. These PDOS have been selected to demonstrates form where the edges states are been generated and which atoms contribute center of the band structure.

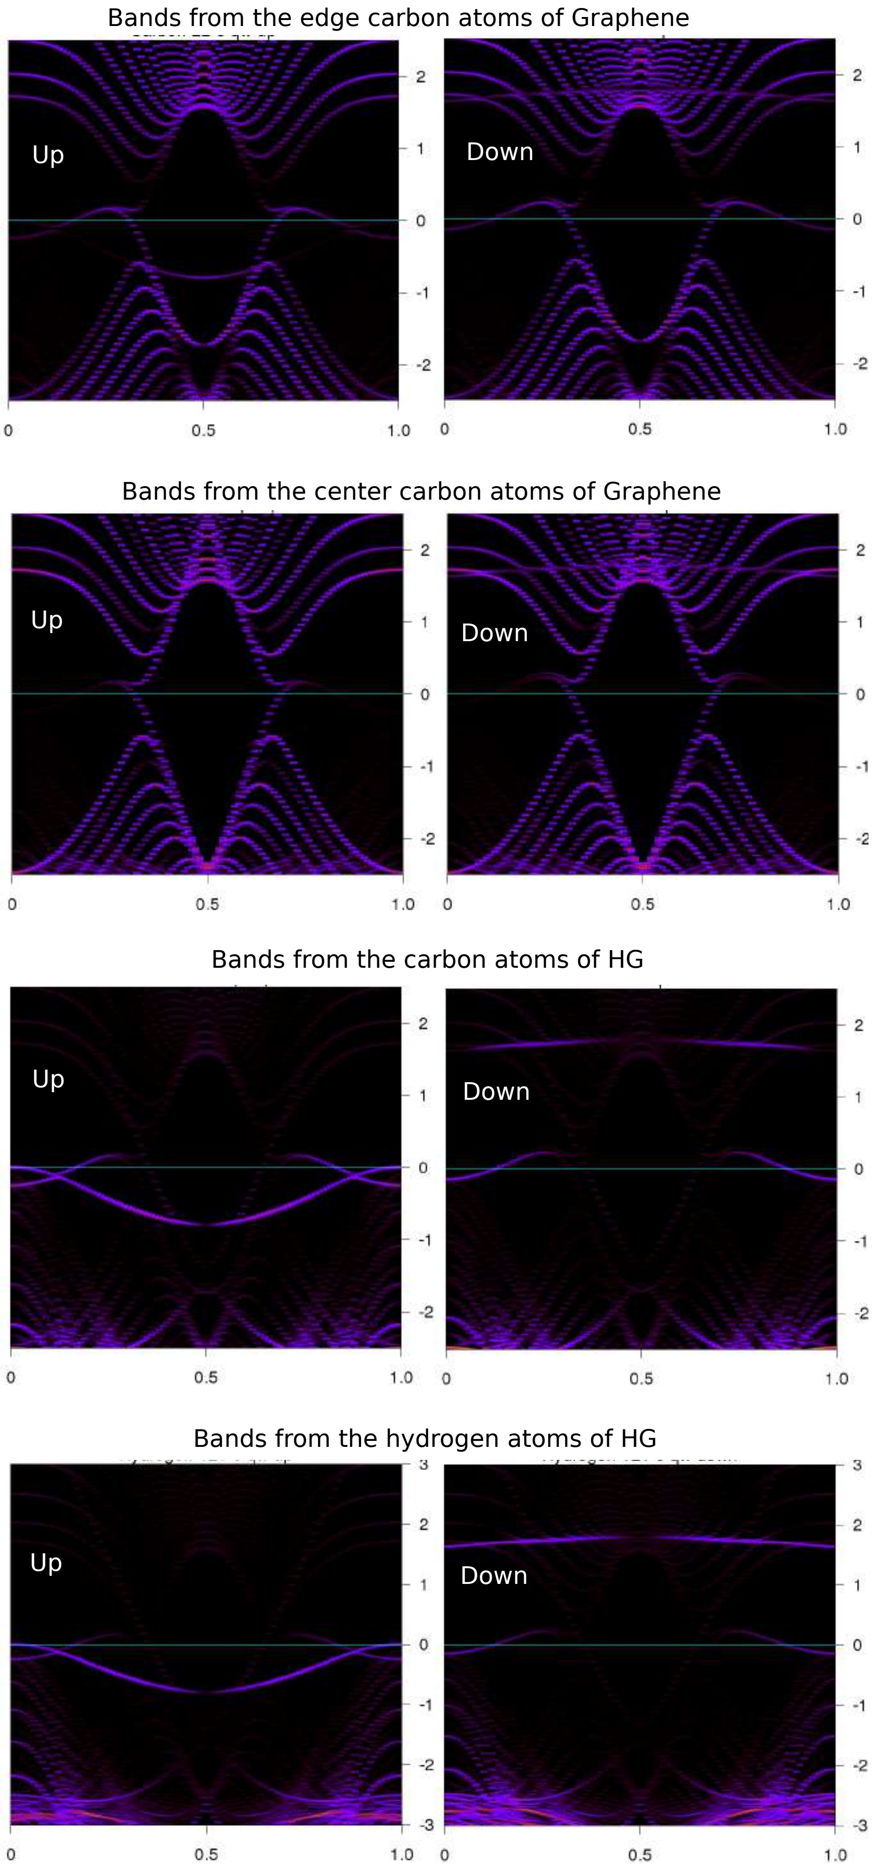


SI: 7: (colour online) $k$-resolved PDOS for the system ZR0

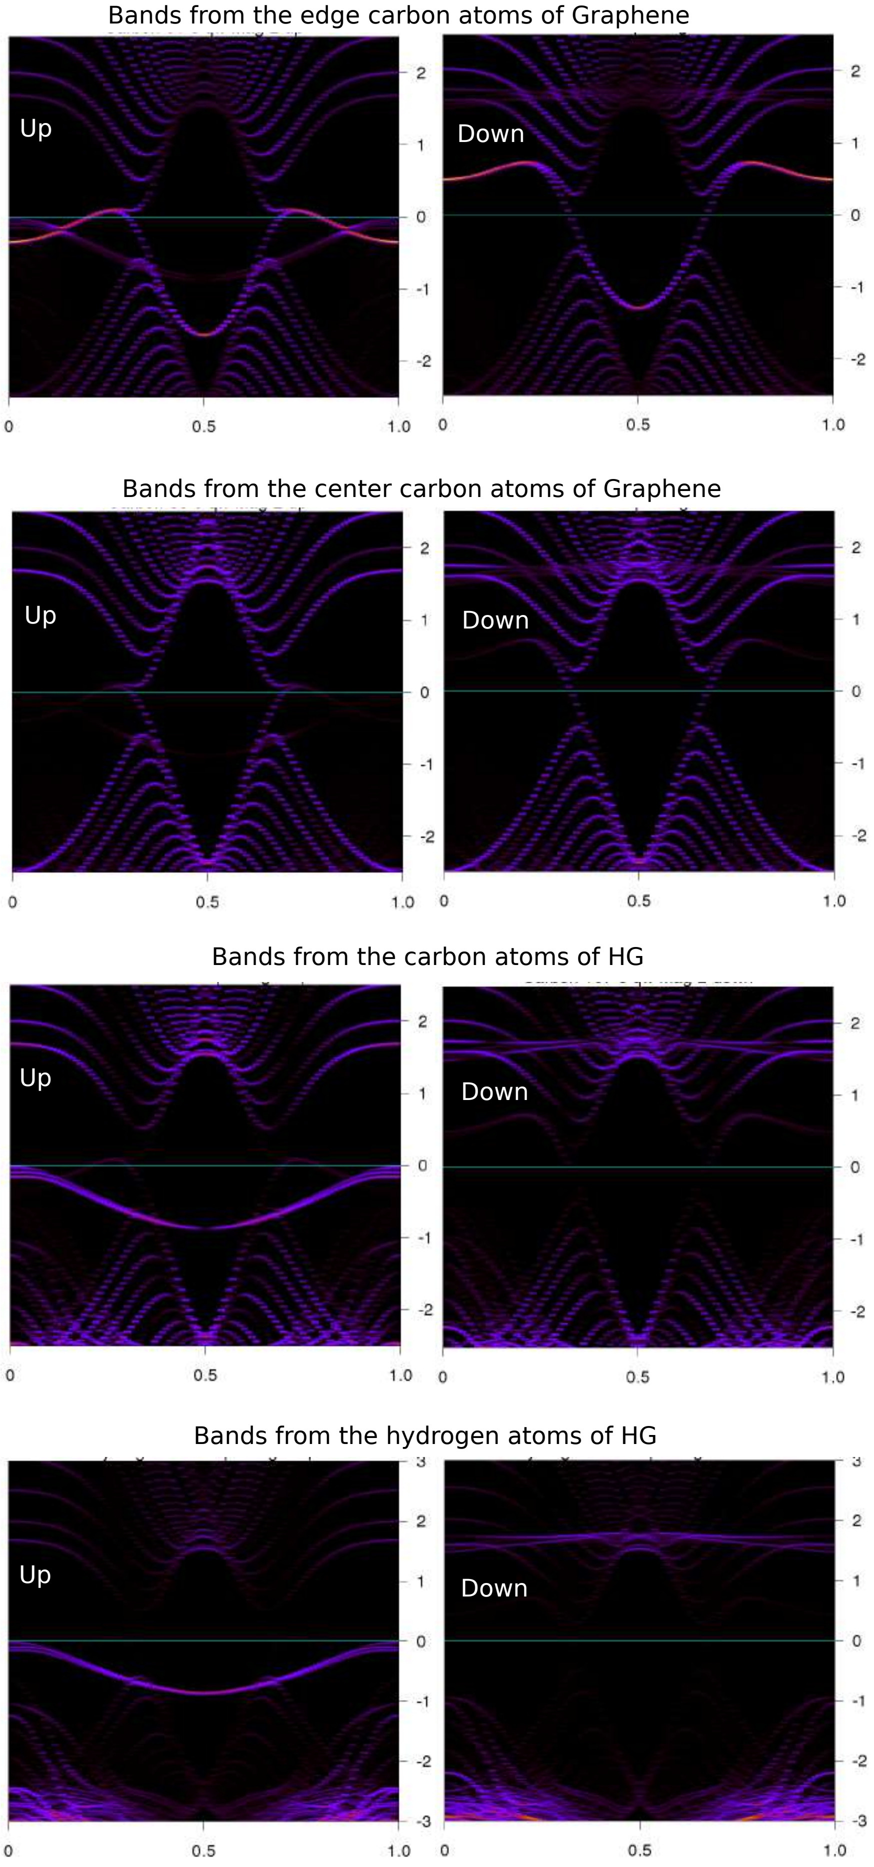


SI: 8: (colour online) $k$-resolved PDOS for the system dis-ZR0

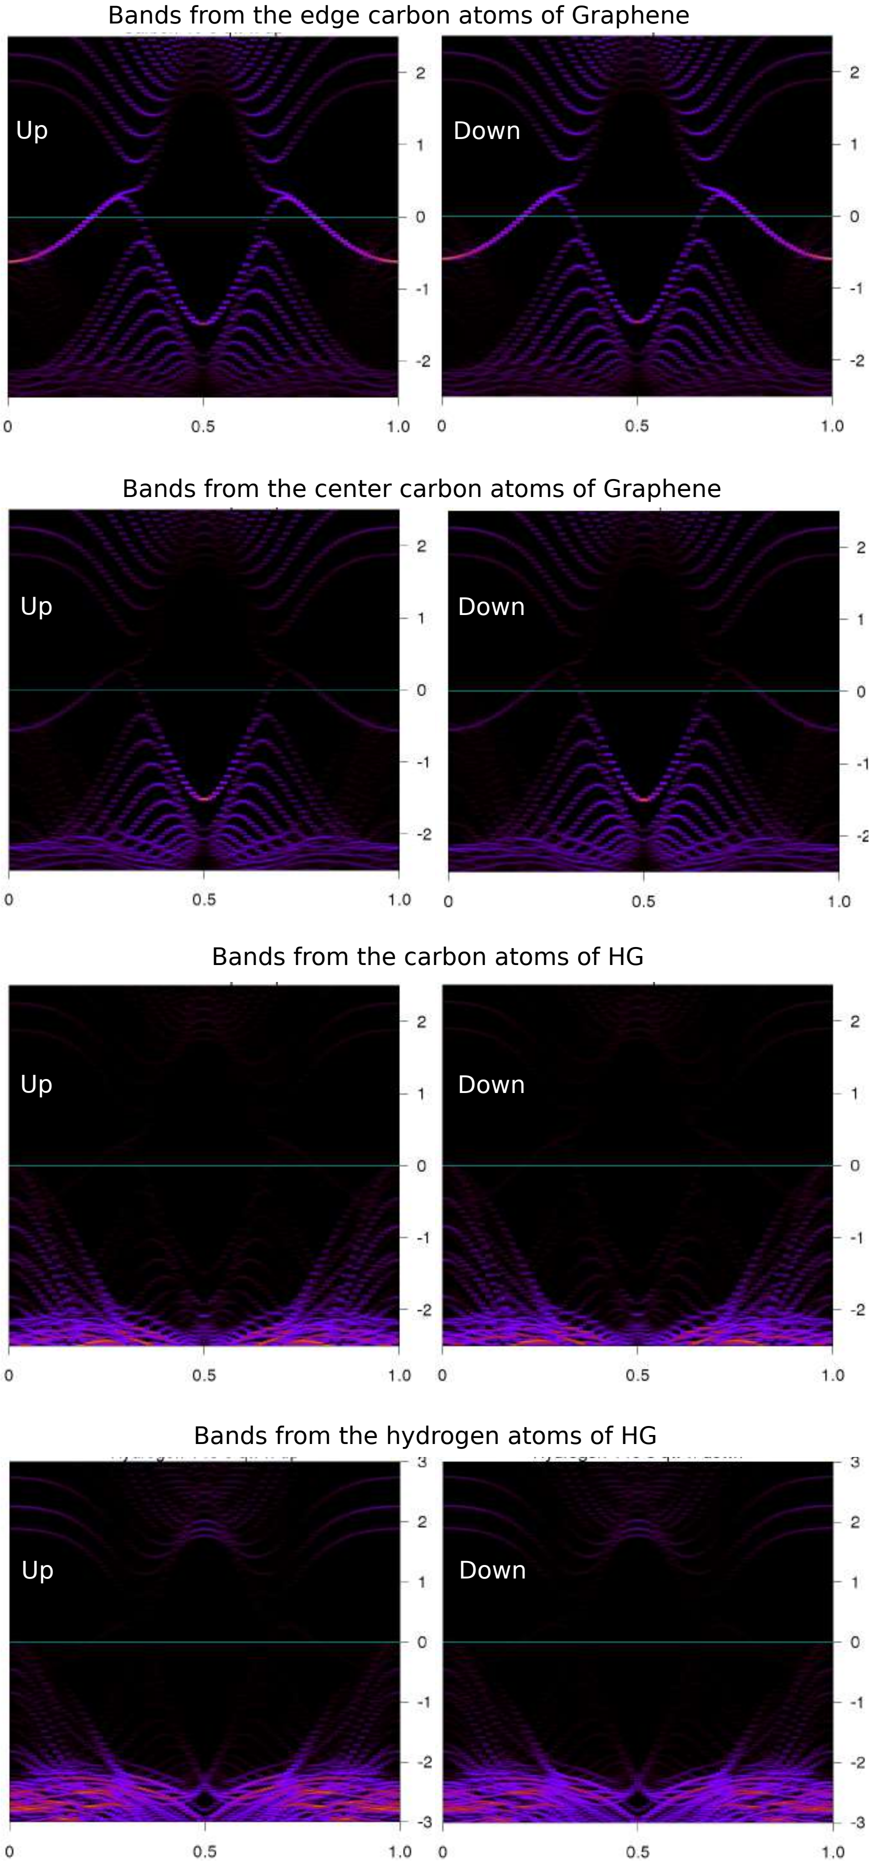


SI: 9: (colour online) $k$-resolved PDOS for the system hydrogenated ZR0

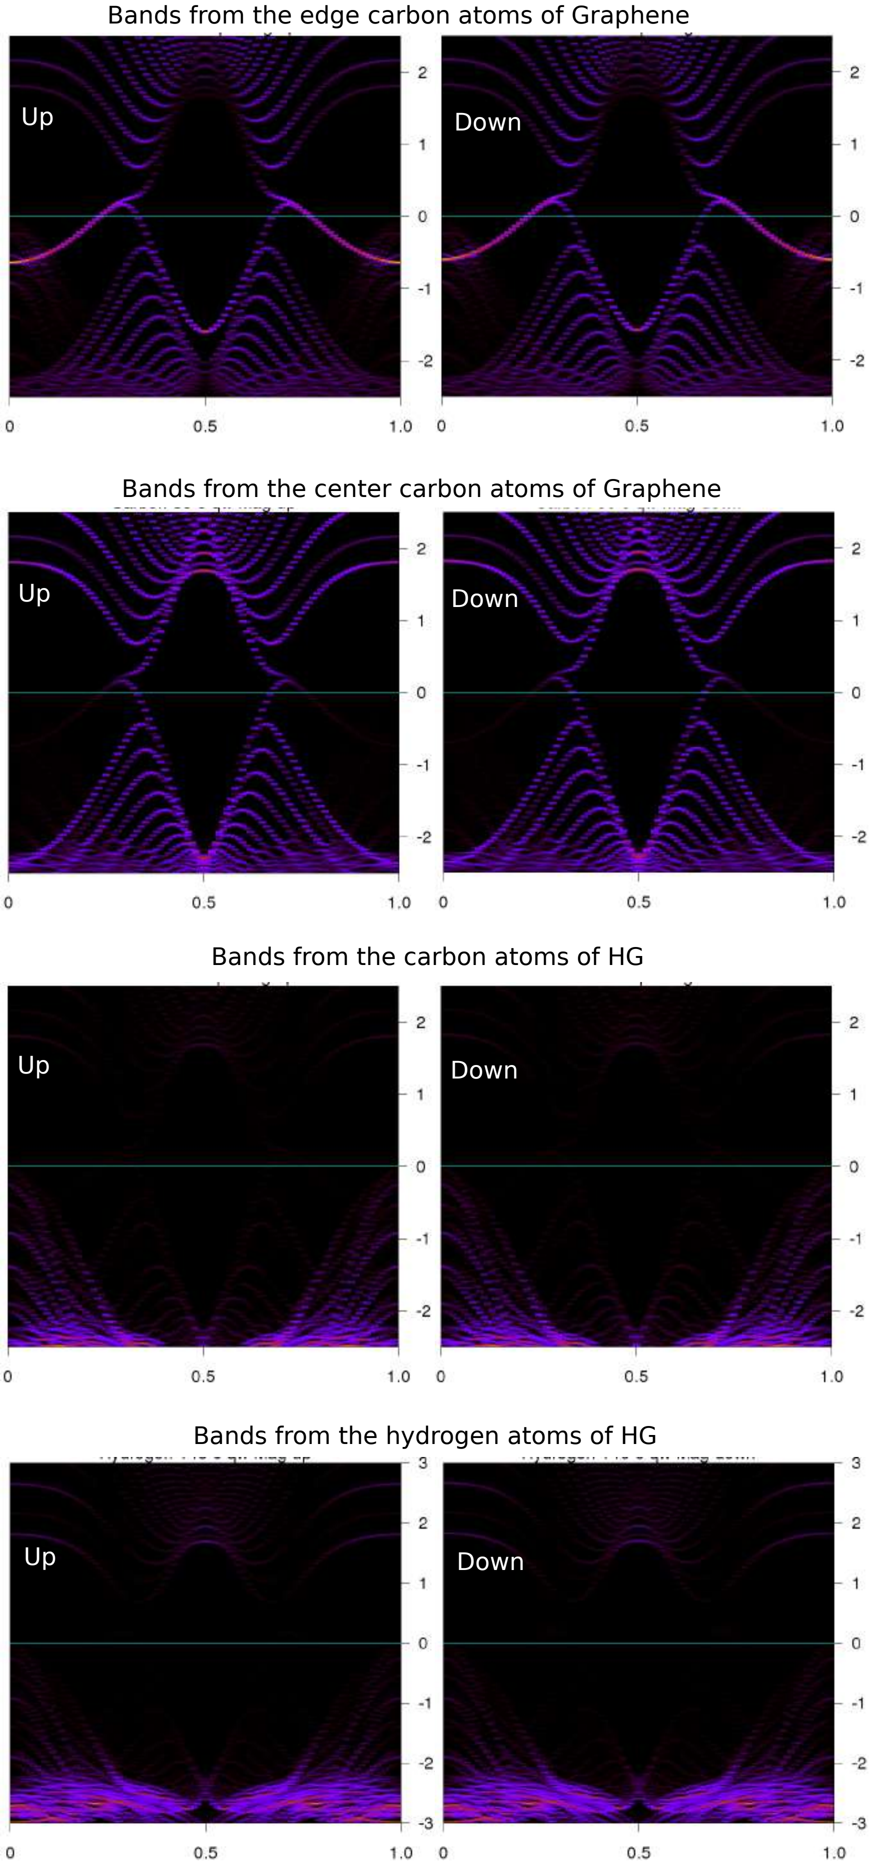


SI: 10: (colour online) $k$-resolved PDOS for the system hydrogenated dis-ZR0.

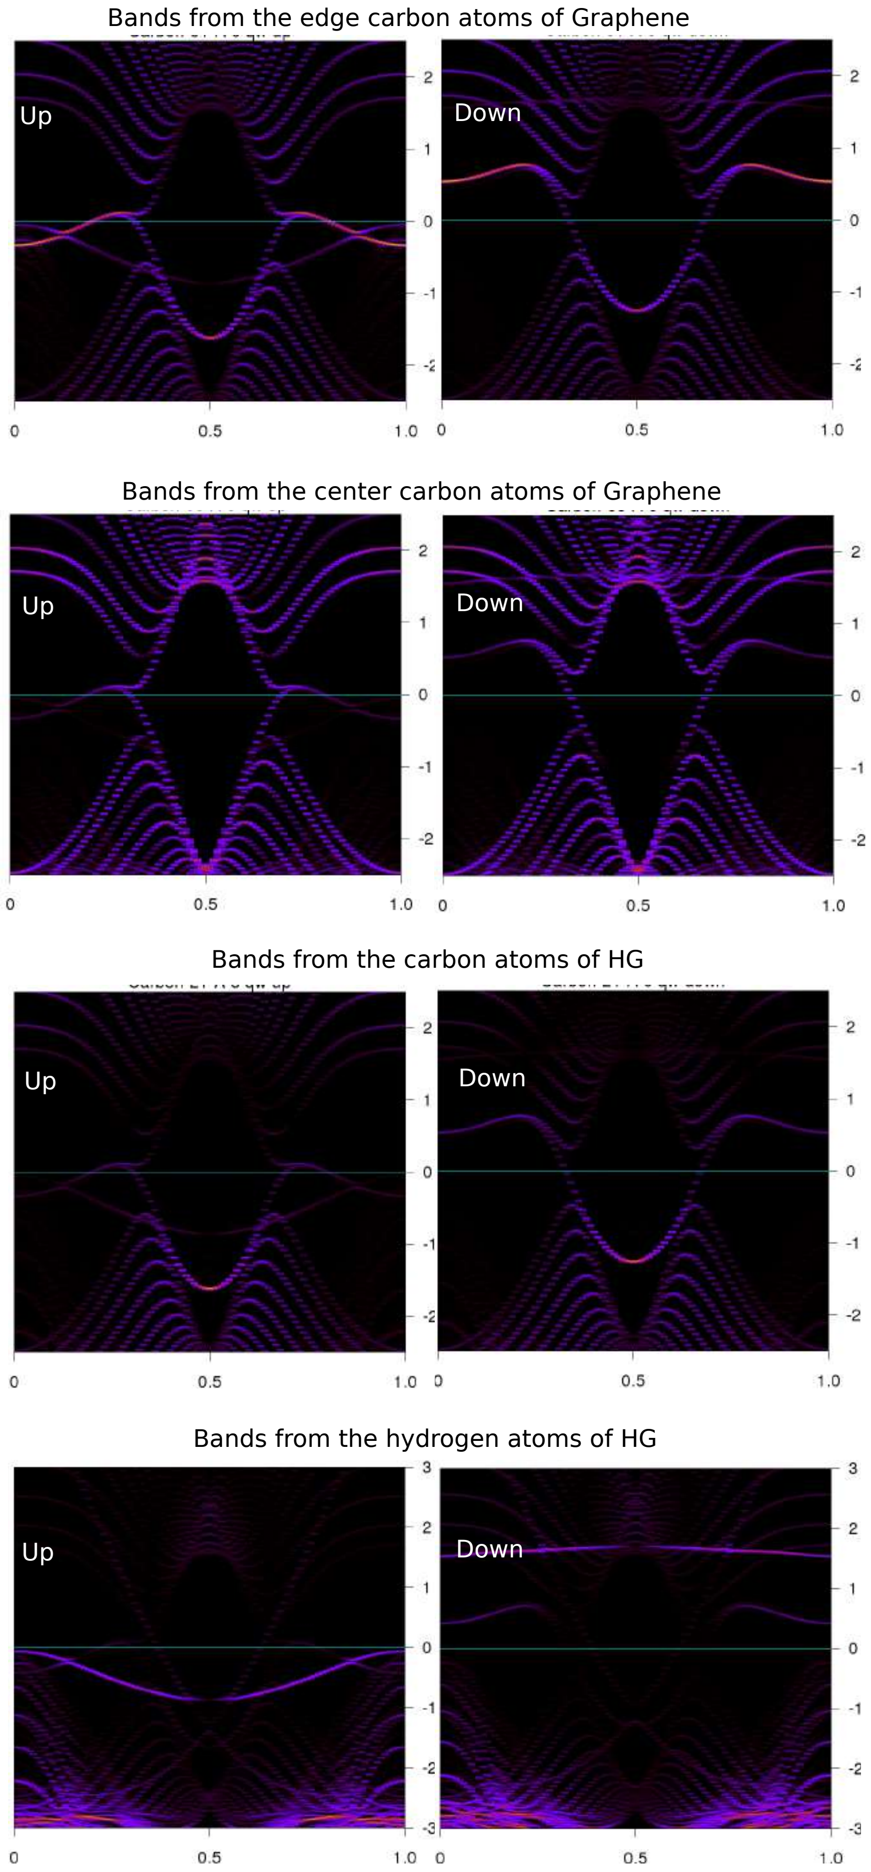


SI: 11: (colour online) $k$-resolved PDOS for the system AR0.

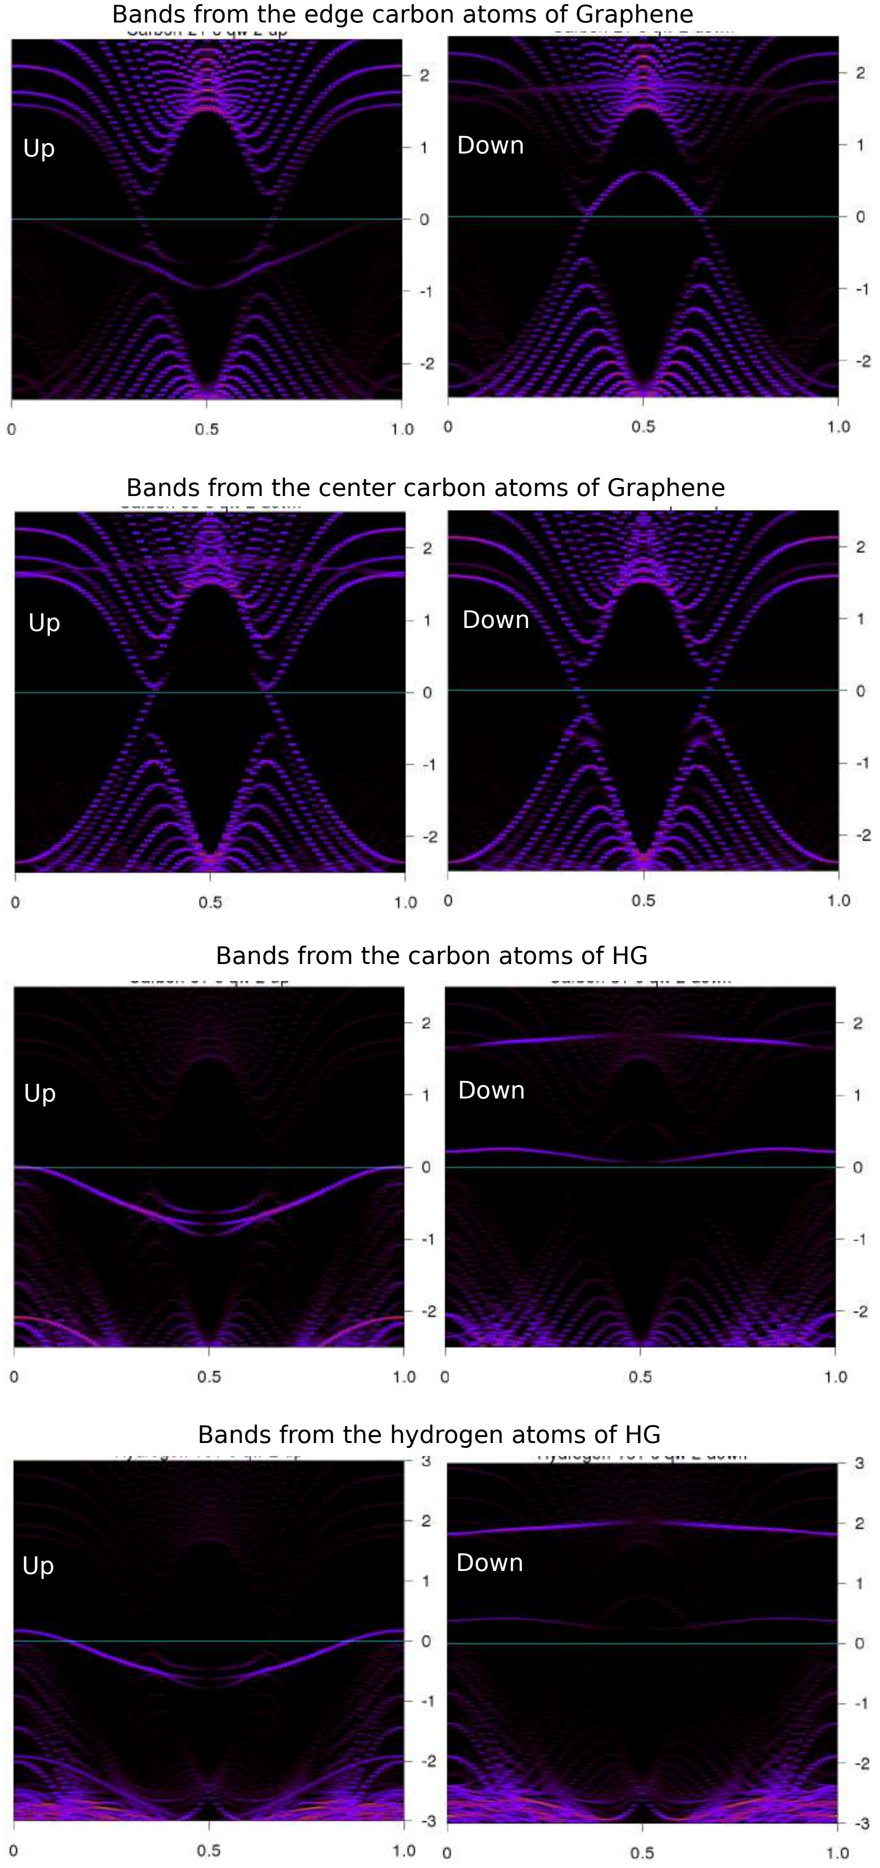


SI: 12: (colour online) $k$-resolved PDOS for the system R60.

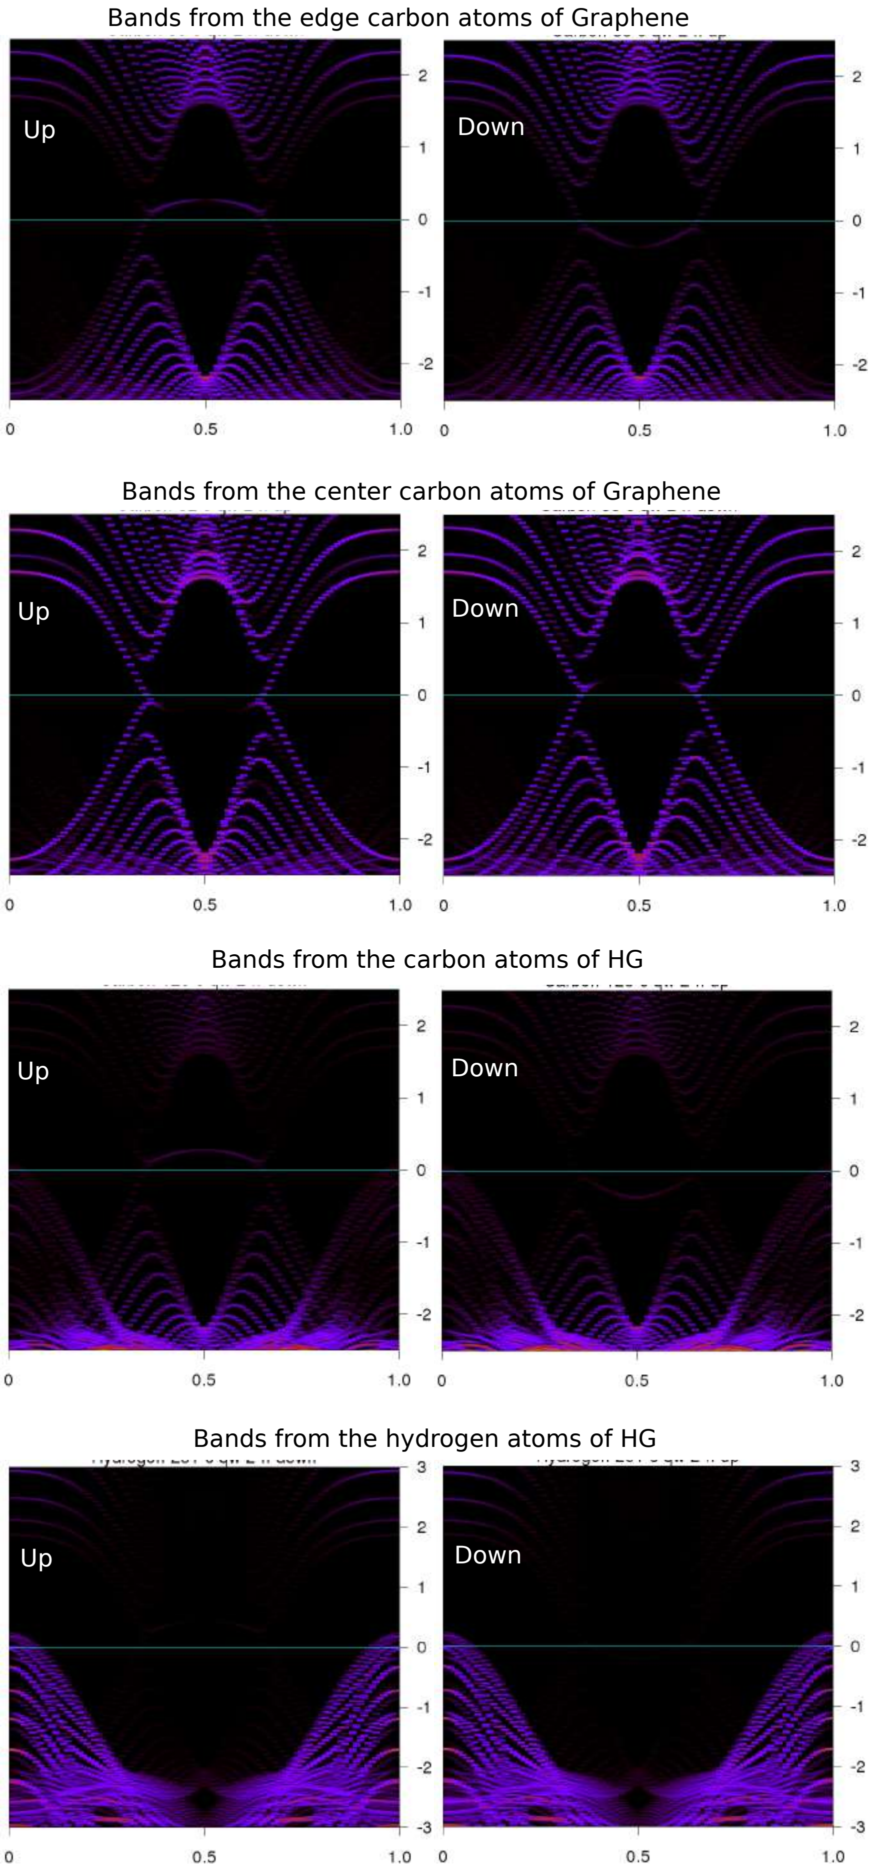


SI: 13: (colour online) $k$-resolved PDOS for the system Hydrogenated R60.

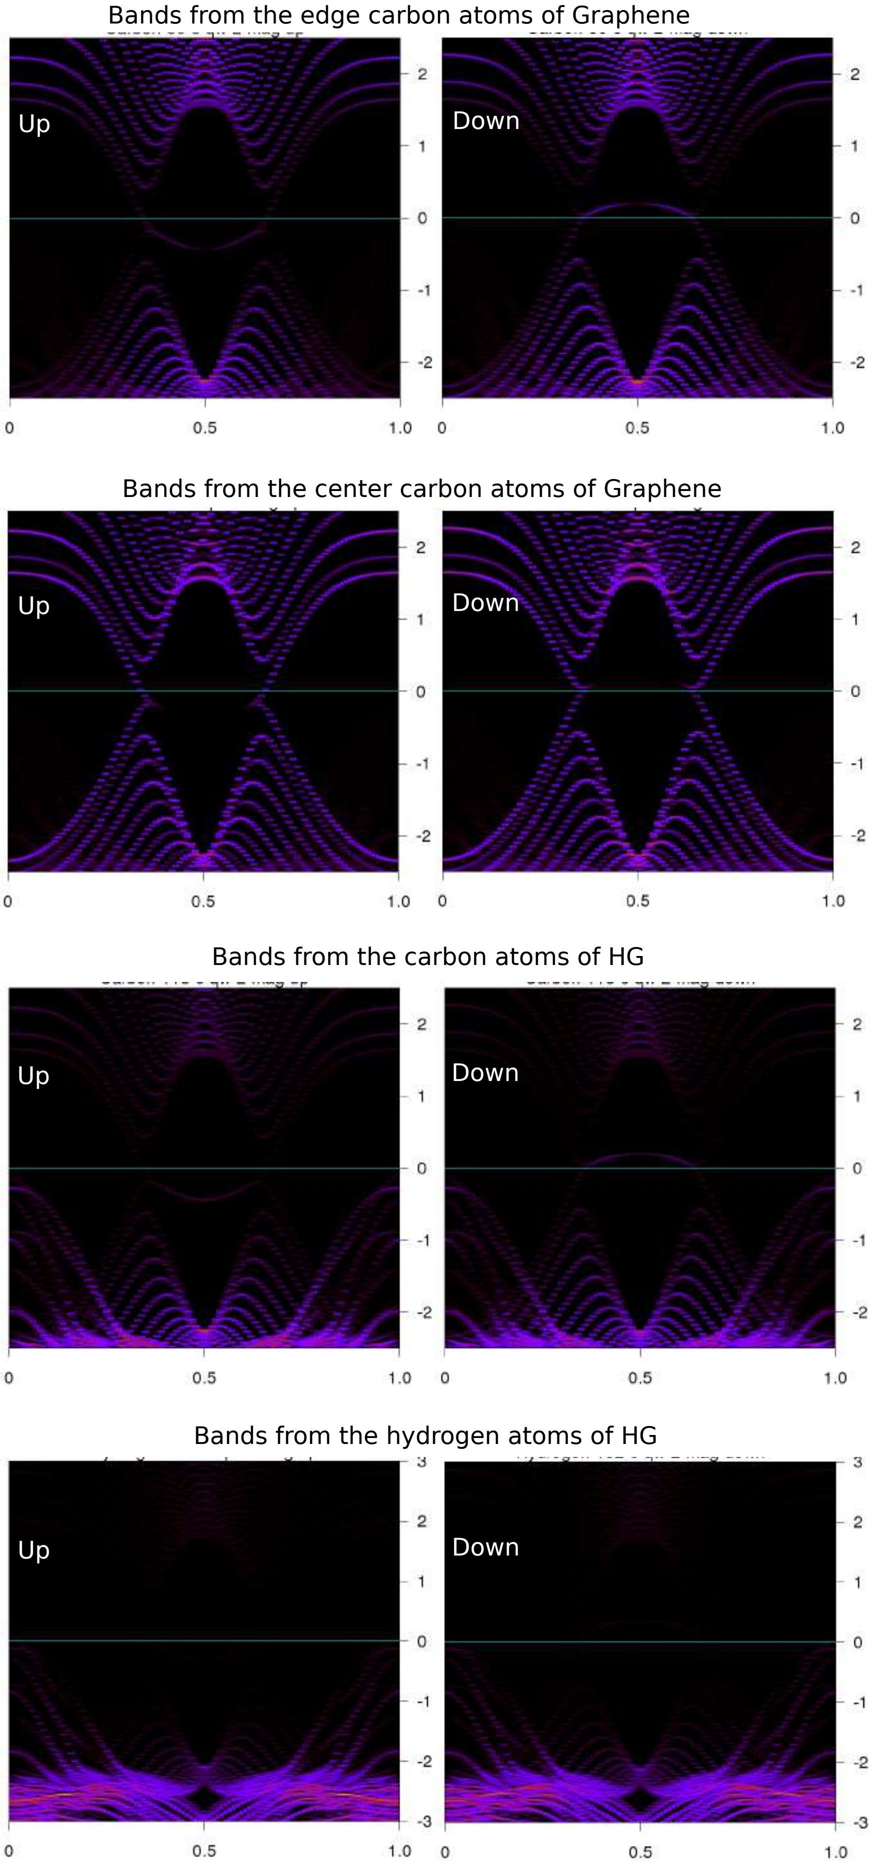


SI: 14: (colour online) $k$-resolved PDOS for the system Hydrogenated dis-R60.

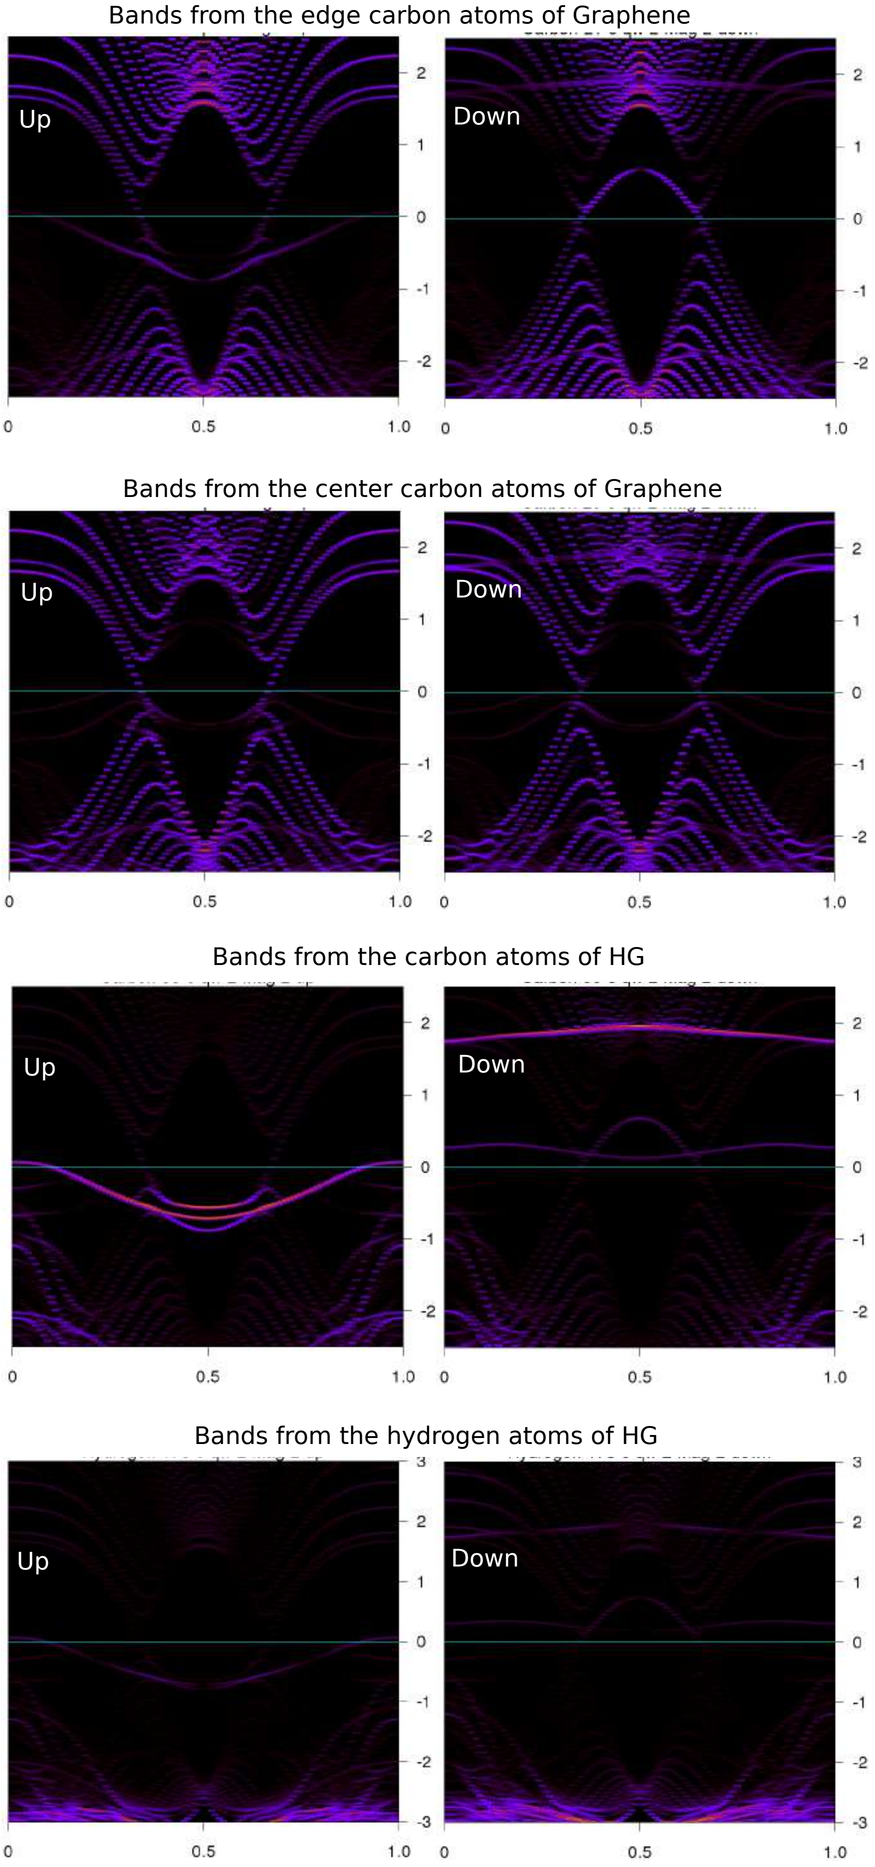


SI: 15: (colour online) $k$-resolved PDOS for the system dis-R60.

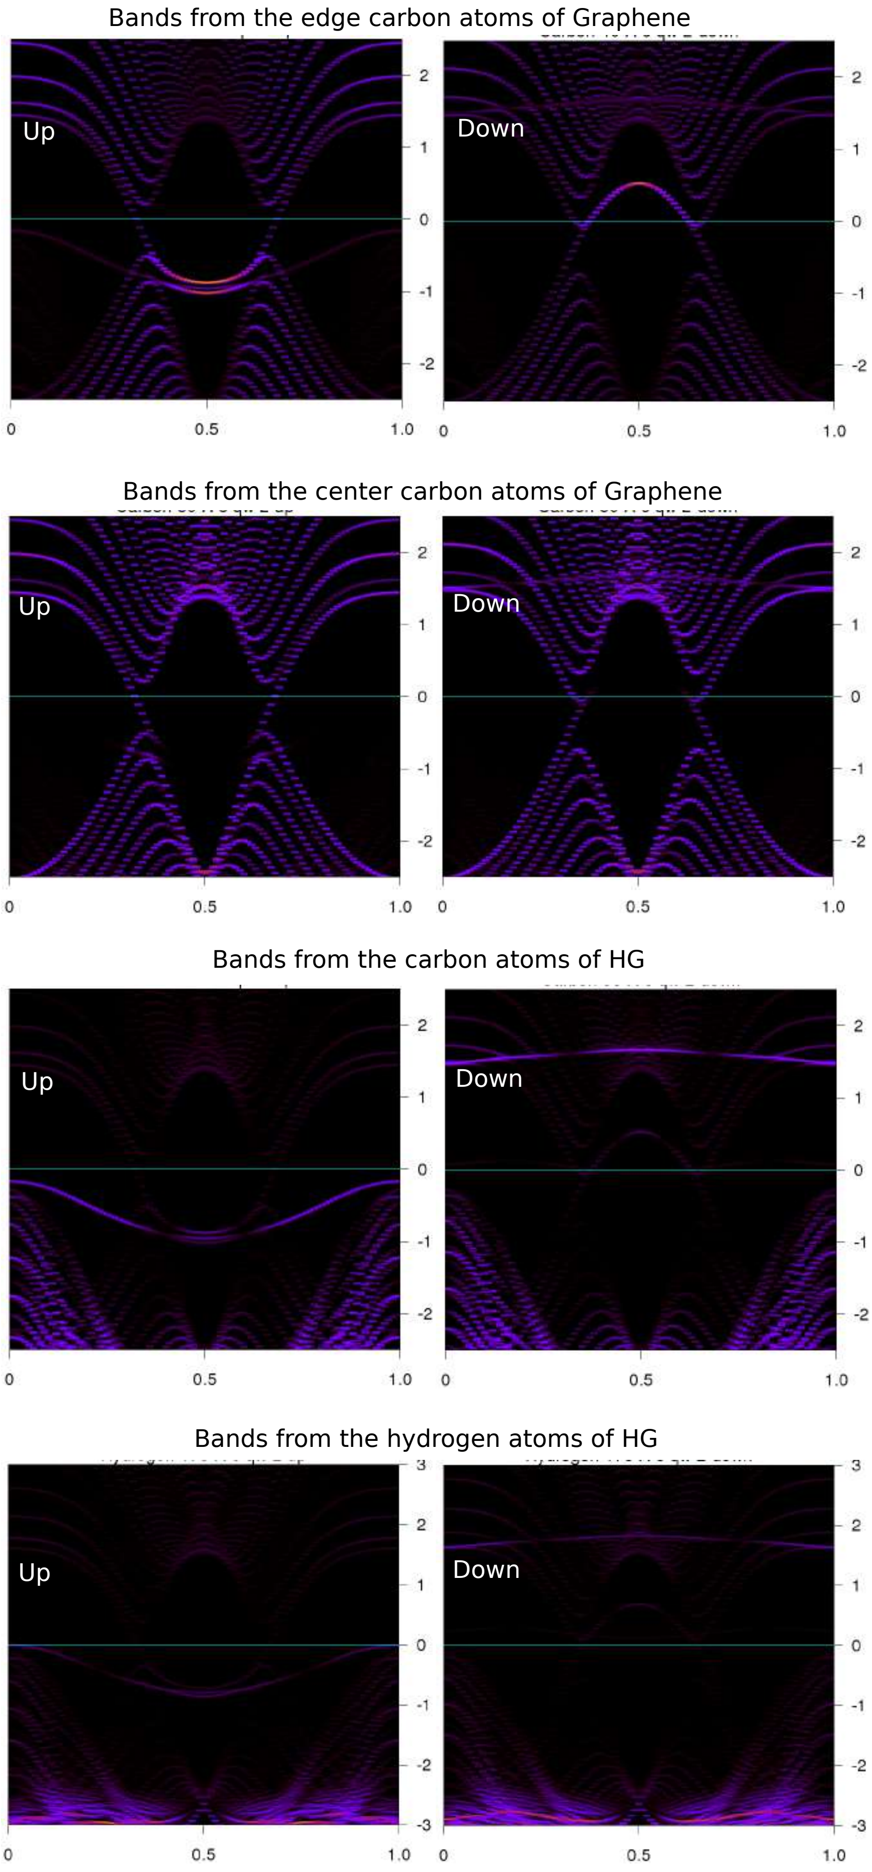


SI: 16: (colour online) $k$-resolved PDOS for the system AR60.

## 6. Bilayer Structures

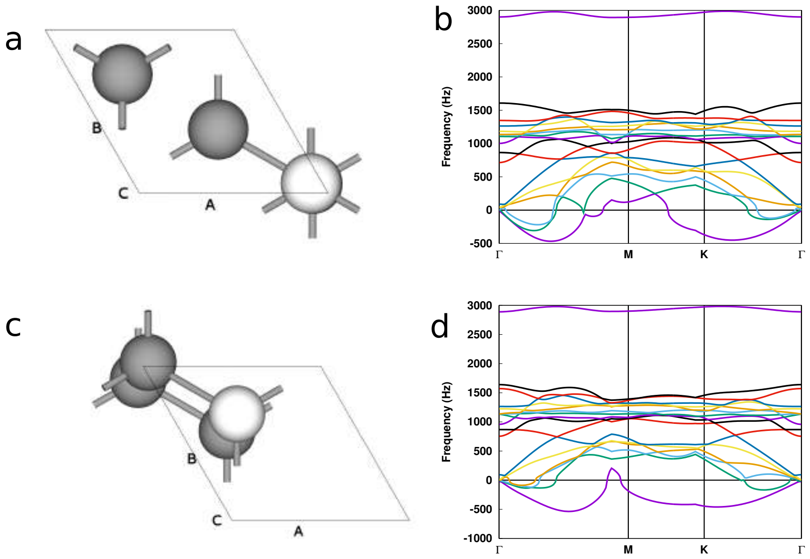


SI: 17: (colour online) (a) and (c) The bilayer structures with very high negative phonon frequencies. They were not studied further due to their unstable structure observed from the high negative phonon frequencies. (b) and (d) are the phonon dispersion of the structures (a) and (c), respectively.

## 7. Band structure of unstable system

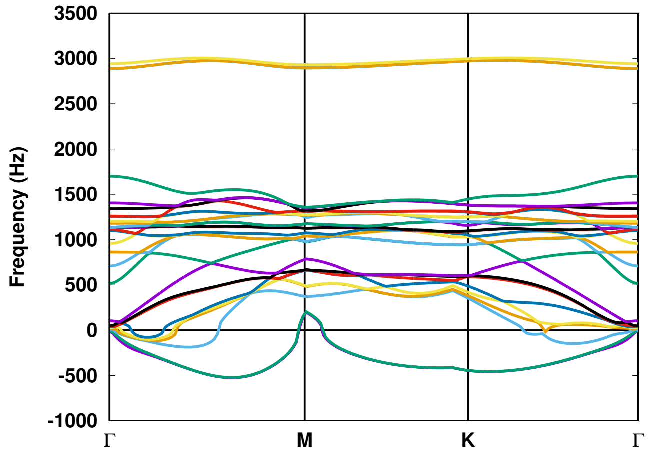


SI: 18: (colour online) The phonon dispersion of the system A0 along the high symmetry k-points, after initial optimization.

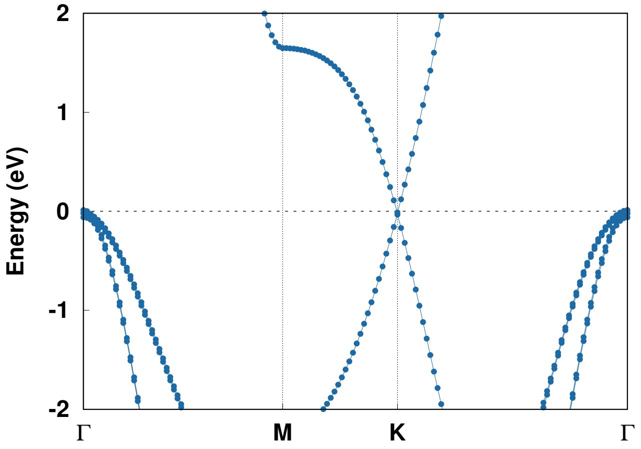


SI: 19: (colour online) Band structure of system A0, after the initial optimization, which exhibits negative phonon dispersion, the image given above 18. It can be noted that difference between band structures of fully optimized structure and initial optimized structure is not very pronounced.
